# Supplementary material for: Boosting Punctuation Restoration with Data Generation and Reinforcement Learning
Source: arXiv:2307.12949 source file (2023-07-24)
Supplement: Supplementary file 1 [file appendix.tex]

\section{Comparison of generated text}

Table \ref{tab:appendix} shows two examples of the generated text by the GPT model after the RL process. 

\begin{table*}[]
    \centering
    \begin{tabular}{|p{8cm}|p{8cm}|}
        \hline
        \multicolumn{2}{|p{16cm}|}{{\bf Input:} ray of hope was born . and I called him luca , which means ``the bringer of light,'' because he does bring light to my life. but I'm talking about him because when he was four months old,...}
        \\ \hline
        {\bf Original text: } \textit{...my foreign editor forced me to go back to Baghdad where I had been reporting all throughout the Saddam regime and during the fall of Baghdad and afterward, and I remember getting on the plane in tears, crying to be separated from my son, and while I was there, a quite famous} 
        & 
        {\bf Generated text: } \textit{...he survived a brain tumor, he survived the chemotherapy and he survived the radiation. he's a survivor. and so i called him my son, and together with him, we decided to build a shelter that would be a little bit more than just a shelter. and we started by building a shelter. and we started by making jewelry. and we made jewelry out of his favorite things, his socks, his purple socks, his shoes, his purple jacuzzi, and he made a purple jacuzzi out of his favorite color, purple socks. and we made a jacuzzi out of his favorite color, purple socks. and we made a jacuzzi out of} 
        \\ \hline
        \multicolumn{2}{|p{16cm}|}{{\bf Input:} — you became a sort of expert in how you lean in. So what did that feel like, and become like in your life? To launch not just a book, not just a best selling ...} 
        \\ \hline
        {\bf Original text: } \textit{..., best viewed talk, but a movement, where people began to literally describe their actions at work as I'm leaning in. ss, I mean, I'm grateful, I'm honored, I'm happy, and it's the very beginning. so I don't know if I'm an expert, or if anyone is an expert. I certainly have done a lot of research. I have read every study, I have pored over the materials, and the lessons are very clear. } 
        & 
        {\bf Generated text: } \textit{... novel, but a career, as you say, into the real world. and what did that look like? well, I think it was exhilarating. I think it was exhilarating because I could see that I was not alone. I was part of a growing cohort of women who were starting to feel that they were not alone in pursuing a career in science, technology, engineering or mathematics. and I think that's a really important thing. I think that's a really important thing because I think that's where the new engineers and the entrepreneurs are going, where they want to start up companies, and I think that's where the people}
        \\ \hline
    \end{tabular}
    \caption{Examples of the original text and generated text.}
    \label{tab:appendix}
\end{table*}
